# Supplementary material for: Dual Anchors, Do It Better: Hierarchical Group Merging for Zero-Shot Anomaly Detection
Source: arXiv:2608.11933 source file (2026-08-12)
Supplement: Supplementary file 1 [file X_suppl.tex]

\clearpage
\onecolumn
\setcounter{page}{1}
\setcounter{section}{0} 
\setcounter{figure}{0}
\setcounter{table}{0}
\maketitlesupplementary
\renewcommand\thesection{\Alph{section}}
\renewcommand\thefigure{S\arabic{figure}}
\renewcommand\thetable{S\arabic{table}}

\section*{Overview}
The supplementary material presents the following sections to strengthen the main manuscript:
\begin{description}
  \item[-- Sec.~\ref{sec:A}] shows more detailed Information, including:
  \begin{itemize}
    \item Sec.~\ref{sec:A1}: Implementation Details,
    \item Sec.~\ref{sec:A2}: Datasets,
    \item Sec.~\ref{sec:A3}: Baseline Methods.
  \end{itemize}
  \item[-- Sec.~\ref{sec:B}] shows additional qualitative results.
  \item[-- Sec.~\ref{sec:C}] shows more analysis, including:
  \begin{itemize}
    \item Sec.~\ref{sec:C1}: Comparison of Computational Efficiency,
    \item Sec.~\ref{sec:C2}: Backbone Comparison,
    \item Sec.~\ref{sec:C3}: Effects of Grouping,
  \end{itemize}
  \item[-- Sec.~\ref{sec:D}] shows Failure Cases.
\end{description}
%%%%%%%%%%%%%%%%%%%%%%%%%%%%%%%%%%%%%%%%%%%%%%%%%%%%%%%%%%%%%%%%%%%%%%%%%%%%%%%%%%%%%%%%%%%%%%%%%%%%%%%%
\section{Detailed Information}
\label{sec:A}

In this section, we first provide additional implementation details, including the hyperparameters used in our model design. We then present dataset statistics and preprocessing protocols for the 8 industrial datasets (MVTec AD~\citep{bergmann2021mvtec}, VisA~\citep{zou2022spot}, MPDD~\citep{jezek2021deep}, BTAD~\citep{mishra2021vt}, RSDD~\citep{yu2018coarse}, KSDD2~\citep{bovzivc2021mixed}, DAGM~\citep{wieler2007weakly}, DTD\text{-}Synthetic~\citep{aota2023zero}) and 6 medical datasets (ISIC~\citep{gutman2016skin}, CVC\text{-}ColonDB~\citep{tajbakhsh2015automated}, CVC\text{-}ClinicDB~\citep{bernal2015wm}, TN3K~\citep{gong2021multi}, Endo~\citep{hicks2021endotect}, Kvasir~\citep{jha2019kvasir}). Finally, we evaluate our method against a variety of vision–language anomaly detection baselines and briefly summarize their key characteristics and implementation details.

%%%%%%%%%%%%%%%%%%%%%%%%%%%%%%%%%%%%%%%%%%%%%%%%%%%%%%%%%%%%%%%%%%%%%
\subsection{Implementation Details}
\label{sec:A1}
\paragraph{Architecture.}
We adopt DINOv3 with a ViT-L/16 backbone as the image encoder. 
To align with the four selected feature layers (6th, 12th, 18th, and 24th), we employ four Hierarchical Merge Blocks. The number of learnable group tokens is initially set to 16 and is progressively 
reduced by a factor of two at each block, resulting in 2 group tokens in the final layer.

\paragraph{Optimization.}
All experiments are conducted on a single NVIDIA GeForce RTX 3090 GPU with 24 GB of memory. 
We train the model for 10 epochs with a batch size of 8, which takes approximately 1 hour in total. 
We use the Adam optimizer with a learning rate of $1\times10^{-4}$ for all experiments.
%%%%%%%%%%%%%%%%%%%%%%%%%%%%%%%%%%%%%%%%%%%%%%%%%%%%%%%%%%%%%%%%%%%%%
\subsection{Datasets}
\label{sec:A2}
\paragraph{MVTec AD~\citep{bergmann2021mvtec}.} The MVTec Anomaly Detection (MVTec AD) dataset is a real-world benchmark for unsupervised visual anomaly detection in industrial inspection. It contains 5,354 high-resolution images from 15 object and texture categories, where 3,629 defect-free images are used for training and 1,725 images with both normal and anomalous samples are used for testing. In total, 73 defect types with pixel-accurate ground-truth masks are provided, enabling evaluation at both image and pixel level.

\paragraph{VisA~\citep{zou2022spot}.}
The VisA dataset is a large-scale industrial visual anomaly detection benchmark consisting of 10{,}821 high-resolution images from 12 object categories across three domains, including printed circuit boards and multi-instance scenes. It contains 9{,}621 normal and 1{,}200 anomalous images with both image- and pixel-level annotations, enabling comprehensive evaluation of detection and localization methods.

\paragraph{MPDD~\citep{jezek2021deep}.}
The Metal Parts Defect Detection (MPDD) dataset targets visual inspection of painted metal parts in real industrial conditions. It comprises about 1.3k images of six types of metal components with pixel-precise defect masks, split into defect-free training images and a validation set containing both normal and defective samples.

\paragraph{BTAD~\citep{mishra2021vt}.}
The BeanTech Anomaly Detection (BTAD) dataset is a real-world industrial anomaly detection benchmark with 2{,}830 RGB images of three industrial products. It includes body and surface defects with a data structure similar to MVTec AD, and is widely used to evaluate industrial anomaly detection and localization methods.

\paragraph{RSDD~\citep{yu2018coarse}.}
The Rail Surface Defect Detection (RSDD) dataset consists of grayscale images captured from express and heavy-haul rails, containing various real rail surface defects such as cracks and squats under challenging outdoor conditions. It is designed to benchmark defect detection and localization methods for rail condition monitoring.

\paragraph{KSDD2~\citep{bovzivc2021mixed}.}
The Kolektor Surface Defect Dataset (KSDD) focuses on detecting defects on electrical commutator surfaces. It contains 399 high-resolution images, including 52 defective and 347 non-defective samples, and is commonly used as a small but challenging benchmark for industrial surface defect segmentation.

\paragraph{DAGM~\citep{wieler2007weakly}.}
The DAGM 2007 dataset is an industrial optical inspection benchmark featuring ten classes of textured surfaces with and without defects. It provides thousands of high-resolution grayscale images with pixel-level ground truth, and is widely used for surface defect detection under complex background textures.

\paragraph{DTD-Synthetic~\citep{aota2023zero}.}
The DTD-Synthetic dataset is a synthetic texture anomaly detection benchmark created by sampling diverse textures from the Describable Texture Dataset (DTD) and injecting artificial defects. It is designed to study zero-shot and few-shot texture anomaly localization under controlled anomaly patterns.

\paragraph{ISIC~\citep{gutman2016skin}.}
The ISIC dataset (International Skin Imaging Collaboration) is a large collection of dermoscopic images of skin lesions, covering multiple diagnostic classes such as melanoma, nevus, and seborrheic keratosis. It provides expert annotations including lesion labels and segmentation masks, and serves as a standard benchmark for skin lesion classification and segmentation.

\paragraph{CVC-ColonDB~\citep{tajbakhsh2015automated}.}
CVC-ColonDB is a colonoscopy dataset composed of 380 still images extracted from 15 colonoscopy videos, each with a corresponding polyp segmentation mask. It is mainly used to evaluate polyp detection and segmentation performance in challenging clinical scenarios.

\paragraph{CVC-ClinicDB~\citep{bernal2015wm}.}
CVC-ClinicDB is a widely used polyp segmentation benchmark consisting of 612 frames extracted from colonoscopy videos collected at Hospital Clínic de Barcelona. Each image is accompanied by a binary ground-truth mask delineating the polyp region at pixel level.

\paragraph{TN3K~\citep{gong2021multi}.}
The TN3K dataset contains 3{,}000 thyroid ultrasound images focusing on the thyroid gland region, with expert annotations of thyroid nodules. It is designed for weakly and fully supervised thyroid nodule detection and segmentation in ultrasound imaging.

\paragraph{Endo~\citep{hicks2021endotect}.}
The Endo dataset is an in-house gastrointestinal endoscopy dataset consisting of endoscopic images with corresponding pixel-level lesion masks. It is used to evaluate anomaly detection and segmentation performance on real clinical endoscopy data.

\paragraph{Kvasir~\citep{jha2019kvasir}.}
The Kvasir-SEG dataset is an open-access gastrointestinal polyp dataset containing 1{,}000 colonoscopy images with corresponding expert-annotated polyp segmentation masks, derived from the Kvasir v2 dataset. It has become a standard benchmark for training and evaluating polyp detection and segmentation models.

%%%%%%%%%%%%%%%%%%%%%%%%%%%%%%%%%%%%%%%%%%%%%%%%%%%%%%%%%%%%%%%%%%%%%
\subsection{Baseline Methods}
\label{sec:A3}
\paragraph{WinCLIP~\citep{WinCLIP}.}
WinCLIP is a window-based CLIP framework for zero- and few-shot anomaly classification and segmentation, which aggregates multi-scale patch features aligned with textual prompts to produce anomaly scores and maps. 

\paragraph{APRIL-GAN~\citep{APRIL-GAN}.}
APRIL-GAN extends CLIP-based anomaly detection by introducing additional adapter layers and a GAN-based refinement module to better map image features into the joint vision–language space for zero-/few-shot anomaly classification and segmentation. 

\paragraph{AnomalyCLIP~\citep{AnomalyCLIP}.}
AnomalyCLIP learns object-agnostic text prompts that represent generic normality and abnormality, enabling CLIP to focus on abnormal regions rather than object semantics for accurate zero-shot anomaly detection across diverse domains. 

\paragraph{AdaCLIP~\citep{AdaCLIP}.}
AdaCLIP adapts CLIP to zero-shot anomaly detection by introducing hybrid learnable prompts, combining static prompts shared across images and dynamic prompts generated per image, which are optimized on auxiliary anomaly detection data. 

\paragraph{AA-CLIP~\citep{AA-CLIP}.}
AA-CLIP enhances zero-shot anomaly detection by making CLIP anomaly-aware via a two-stage adaptation that first constructs anomaly-aware text anchors and then aligns patch-level visual features with these anchors using lightweight residual adapters. 

\paragraph{Bayes-PFL~\citep{Bayes-PFL}.}
Bayes-PFL formulates prompt learning for zero-shot anomaly detection in a Bayesian manner, modeling prompts as distributions and using Monte Carlo sampling over prompt flows to improve robustness and generalization across categories and domains. 

%%%%%%%%%%%%%%%%%%%%%%%%%%%%%%%%%%%%%%%%%%%%%%%%%%%%%%%%%%%%%%%%%%%%%
\section{Additional Qualitative Results}
\label{sec:B}
% mvtec
\input{suppl_figure/mvtec/bottle/bottle}
\input{suppl_figure/mvtec/capsule/capsule}
\input{suppl_figure/mvtec/carpet/carpet}
\input{suppl_figure/mvtec/grid/grid}
\input{suppl_figure/mvtec/hazelnut/hazelnut}
\input{suppl_figure/mvtec/leather/leather}
\input{suppl_figure/mvtec/metal_nut/metal_nut}
\input{suppl_figure/mvtec/screw/screw}
\input{suppl_figure/mvtec/tile/tile}
\input{suppl_figure/mvtec/wood/wood}
\input{suppl_figure/mvtec/zipper/zipper}

% visa
\input{suppl_figure/visa/candle/candle}
\input{suppl_figure/visa/capsules/capsules}
\input{suppl_figure/visa/cashew/cashew}
\input{suppl_figure/visa/chewinggum/chewinggum}
\input{suppl_figure/visa/fryum/fryum}
\input{suppl_figure/visa/macaroni1/macaroni1}
\input{suppl_figure/visa/pipe_fryum/pipe_fryum}
%%%%%%%%%%%%%%%%%%%%%%%%%%%%%%%%%%%%%%%%%%%%%%%%%%%%%%%%%%%%%%%%%%%%%
\clearpage
\section{Additional Analysis of Efficiency, Backbones, and Group Merging}
\label{sec:C}
\subsection{Comparison of Computational Efficiency}
\label{sec:C1}
\input{suppl_table/computation_table}
Table~\ref{tab:s1} compares the computational efficiency of our method with existing vision–language anomaly detection baselines in terms of GPU memory usage, training time per epoch, and inference time. All metrics are measured with a batch size of 1, and all methods are trained on the VisA dataset and evaluated on the MVTec AD dataset. AnomalyCLIP shows the lowest training memory footprint (2.90~GB) and fastest inference (12.5~ms), but its detection performance is clearly inferior to later methods. AdaCLIP and Bayes-PFL require substantially more memory (10.55~GB and 14.90~GB, respectively) and much longer training time, while still underperforming our approach. In contrast, our method achieves competitive efficiency, using only 4.58~GB of memory and 3:33 minutes per epoch with an average inference time of 148.0~ms, while attaining the best image-level and pixel-level results (92.7/94.0/97.1 and 92.4/50.4). These results indicate that our framework strikes a favorable balance between computational cost and anomaly detection performance.


\subsection{Backbone Comparison: CLIP, DINOv2, and DINOv3}
\label{sec:C2}
\input{suppl_table/backbone_table}
As mentioned earlier, we adopt DINOv3~\citep{simeoni2025dinov3} as our image encoder. We make this choice for the following reasons. First, DINOv3 provides richer visual representations than the CLIP image encoder~\citep{CLIP}, which is beneficial for capturing fine-grained semantic cues in images. However, since DINOv3 is not explicitly aligned with text features, it can be less favorable for conventional zero-shot vision-language tasks. In our setting, we deliberately favor the former aspect of this trade-off: our primary objective is to construct an image anchor that reduces dependence on text features and to learn image representations that are semantically meaningful on their own. In this context, DINOv3 is a natural choice, as it allows us to exploit strong visual semantics while shifting the burden away from text-guided supervision. Moreover, aligning DINO-style visual features with text features is itself a non-trivial problem that has been treated as a separate research task in prior work~\citep{jose2025dinov2, barsellotti2025talking}. Building such alignment into our framework is a key component of our method and constitutes an essential part of our novelty.

Despite these considerations, we also compare against the original CLIP-based setting to ensure a fair evaluation. As shown in Table~\ref{tab:s2}, CLIP, DINOv2, and DINOv3 have comparable numbers of parameters, yet our method consistently outperforms most existing approaches even when we replace the image encoder with CLIP or DINOv2, when training on the MVTec AD dataset and evaluating on the VisA dataset. This result not only demonstrates the robustness of our framework to the choice of backbone, but also suggests that future advances in image encoders can be readily leveraged to further improve our model’s performance. 

\subsection{Effects of Hierarchical Group Merging}
\label{sec:C3}
\input{suppl_figure/attn/attn}
The novelty of the proposed \textit{Hierarchical Group Merging} can be summarized as follows. 
(1) Instead of treating patch features from the backbone network as independent tokens without explicit normal/anomaly semantics, our top-down grouping strategy progressively aggregates them into semantically meaningful normal and anomaly groups. This allows the model to form image-level semantic features that are independent of text prompts. 
(2) By ultimately constructing an image anchor, our method reduces the reliance on text anchors and facilitates the formation of a more robust decision boundary in unseen domains. 
To validate these advantages, in this section we compare the attention maps extracted from vanilla CLIP and DINOv3 with those obtained from our \textit{Hierarchical Group Merging}.

Figure~\ref{fig:attn} qualitatively compares the attention maps of our \textit{Hierarchical Group Merging} with those of CLIP, DINOv2, and DINOv3. For the baselines, we extract attention from the same layer used for patch tokens, using the CLS token as the query. While these backbone features produce noisy and scattered responses across levels, our merge block, which is built on hierarchically grouped tokens, progressively concentrates attention on the true anomalous region and yields compact maps that better align with the ground-truth defect.


%%%%%%%%%%%%%%%%%%%%%%%%%%%%%%%%%%%%%%%%%%%%%%%%%%%%%%%%%%%%%%%%%%%%%
\section{Failure Cases}
\label{sec:D}
\input{suppl_figure/failure_case/failure_case}
Figure~\ref{fig:fail} illustrates a representative failure case. 
Due to the zero-shot setting, our model sometimes struggles with logical anomalies that do not manifest as clear low-level appearance changes, such as ``misplaced'' or subtly shifted components in unseen domains. 
In such cases, the visual evidence is weak and the anomaly can only be identified by understanding the global layout or functional semantics of the scene, which goes beyond what our image anchor is explicitly trained to capture. 
We note, however, that other zero-shot anomaly detection methods (e.g., AnomalyCLIP, AdaCLIP, and Bayes-PFL) exhibit similar failure patterns on this example, suggesting that handling such high-level logical anomalies remains an open challenge for zero-shot AD in general.
